# Supplementary material for: Diffusion-based Aesthetic QR Code Generation via Scanning-Robust Perceptual Guidance
Source: arXiv:2403.15878 source file (2024-03-23)
Supplement: Supplementary file 1 [file supp.tex]

\newpage

\begin{center}
\LARGE{\textbf{Supplementary Material}}
\end{center}

\section{Image Processing Operators}
\subsection{Gray-scale Conversion}
We denote $\mathcal{G}(\cdot)$ as the gray-scale operator, which is defined as:
\begin{align}
    \mathcal{G}(\mathbf{x}) =
    c_r \mathbf{x}^r +
    c_g \mathbf{x}^g +
    c_b \mathbf{x}^b,
\end{align}
where $\mathbf{x}^r, \mathbf{x}^g, \mathbf{x}^b$ represent the $R$, $G$, $B$ channel of image $\mathbf{x}$ respectively, and the coefficient are given by $c_r=0.299$, $c_g=0.587$, $c_b=0.114$, which follows the YCbCr color space gray-scale conversion.

\subsection{Binarization}
We denote $\mathcal{B}(\cdot)$ as the binary operator, which is defined as:
\begin{align}
    \mathcal{B}(\mathbf{x}_{i, j}) =
    \begin{cases}
        1, \text{ if } \mathcal{G}(\mathbf{x}_{i, j}) \geq \frac{1}{2} \\
        0, \text{ if } \mathcal{G}(\mathbf{x}_{i, j}) < \frac{1}{2}.
    \end{cases}
\end{align}

\section{Scanning-Robust Perceptual Guidance (SRPG)}
\subsection{Learned Perceptual Image Patch Similarity (LPIPS)}
In evaluating image similarity, conventional metrics mainly focus on the statistical characteristics of image pixels, however, these metrics often fall short of reflecting the real scenarios in human perception. Zhang et al. \cite{zhang2018unreasonable} proposed a new paradigm in leveraging pre-trained NN-based feature extractors, e.g., VGG, AlexNet to transform the image to feature space for comparison, aiming to simulate the high-level human perception. Since our goal is to ensure the ``aesthetics'', which is a relatively high-level and abstract semantic, we adopt LPIPS here for better constraint.  Specifically, the $ \mathcal{L}_\text{LPIPS}(\mathbf{x}, \hat{\mathbf{x}}) $ is defined as:

\begin{align}
    \mathcal{L}_\text{LPIPS}(\mathbf{x}, \hat{\mathbf{x}}) =
    \sum_{l, i, j} \frac{1}{h_l w_l}
    \| \omega^l \odot (\psi^l(\mathbf{x})_{i, j}-\psi^l(\hat{\mathbf{x}})_{i, j}) \|_2^2,
\end{align}
where $\psi^l(\mathbf{x})$ is the feature extracted by layer $l$, $\omega^l$ is channel-wise scale vector, $h_l, w_l$ be the height and width of $\psi^l(\mathbf{x})$.

\subsection{Conditional Probability Derivation of Generalized Classifier Guidance}
Song et al. \cite{song2019generative, song2020score} bridge the score function $\nabla_{\mathbf{z}_t} \log p(\mathbf{z}_{t})$ with the noise estimation $\epsilon_\theta(\mathbf{z}_t, t, \mathbf{e}_p, \mathbf{e}_\text{code})$ via Tweedie's Formula \cite{efron2011tweedie}
\begin{align*}
    \epsilon_\theta(\mathbf{z}_t, t, \mathbf{e}_p, \mathbf{e}_\text{code})
    = -{\sqrt{1-\bar{\alpha}_t}}
    \nabla_{\mathbf{z}_t} \log p(\mathbf{z}_{t}).
\end{align*}
Inspired by \cite{dhariwal2021diffusion}, to perform conditional sampling, we substitute the score function with conditional probability $p(\mathbf{z}_t | \mathbf{y})$. Then we rewrite the conditional probability $p(\mathbf{z}_t | \mathbf{y})$ using Bayes' Theorem. Specifically, we define the updated score estimate $\hat{\epsilon}_t$ of timestep $t$ with condition $\mathbf{y}$ as:
\begin{align*}
    \hat{\epsilon}_t
    &:=-{\sqrt{1-\bar{\alpha}_t}}
    \nabla_{\mathbf{z}_t} \log p(\mathbf{z}_t | \mathbf{y}) \\
    &= -{\sqrt{1-\bar{\alpha}_t}}
    \nabla_{\mathbf{z}_t} \log 
    \left( \frac{p(\mathbf{z}_t)p(\mathbf{y}|\mathbf{z}_{t})}{p(\mathbf{y})}\right) \\
    &= -{\sqrt{1-\bar{\alpha}_t}}
    \left(\nabla_{\mathbf{z}_t} \log p(\mathbf{z}_t)
    +\nabla_{\mathbf{z}_t} \log p(\mathbf{y}|\mathbf{z}_{t}) \right) \\
    & = \epsilon_\theta(\mathbf{z}_t, t, \mathbf{e}_p, \mathbf{e}_\text{code})
    -{\sqrt{1-\bar{\alpha}_t}}
    \nabla_{\mathbf{z}_t} \log p(\mathbf{y}|\mathbf{z}_{t}).
\end{align*}

\subsection{Derivation of SRPG Gradient}
In this section, we derive our Scanning-Robust Perceptual Guidance (SRPG). 
Since $\mathbf{x}_{0|t} = \mathcal{D}_{\theta}
    \left(\frac{1}{\sqrt{\bar{\alpha}_t}}\left(\mathbf{z}_t - \sqrt{1-\bar{\alpha}_t}
    \epsilon_\theta(\mathbf{z}_t, t, \mathbf{e}_p, \mathbf{e}_\text{code})\right)\right)$ 
which involves the VAE decoder calculation, we need to follow the Chain Rule for the derivation. 
Therefore, the gradient of our proposed generalized classifier guidance function $F_\text{SRP}$ can be derived as follows:
\begin{align*}
    \nabla_{\mathbf{z}_t} F_\text{SRP}(\mathbf{z}_t, \mathbf{y}, \hat{\mathbf{x}})
    &=\lambda_1 \nabla_{\mathbf{z}_t} \mathcal{L}_\text{SR}(\mathbf{x}_{0|t}, \mathbf{y}) +
    \lambda_2 \nabla_{\mathbf{z}_t} \mathcal{L}_\text{LPIPS}(\mathbf{x}_{0|t}, \hat{\mathbf{x}}) \\
    &= \left(\lambda_1 \frac{\partial \mathcal{L}_\text{SR}(\mathbf{x}_{0|t}, \mathbf{y})}{\partial \mathbf{x}_{0|t}} + \lambda_2 \frac{\partial \mathcal{L}_\text{LPIPS}(\mathbf{x}_{0|t}, \hat{\mathbf{x}})}{\partial \mathbf{x}_{0|t}} \right) \cdot
    \frac{\partial \mathcal{D}_{\theta}(\mathbf{z}_{0|t})}{\partial \mathbf{z}_{0|t}} \cdot \\
    & \hspace{3cm} \frac{1}{\sqrt{\bar{\alpha}_t}}\left(1 - \sqrt{1-\bar{\alpha}_t} \frac{\partial
    \epsilon_\theta(\mathbf{z}_t, t, \mathbf{e}_p, \mathbf{e}_\text{code})}{\partial\mathbf{z}_t}\right).
\end{align*}

Substitute the conditional score term with $F_\text{SRP}(\mathbf{z}_t, \mathbf{y}, \hat{\mathbf{x}})$, the estimated score of timestep $t$ therefore becomes: 
\begin{align*}
    \hat{\epsilon}_t
    = \epsilon_\theta(\mathbf{z}_t, t, \mathbf{e}_p, \mathbf{e}_\text{code})
    +{\sqrt{1-\bar{\alpha}_t}}
    \nabla_{\mathbf{z}_t} F_\text{SRP}(\mathbf{z}_t, \mathbf{y}, \hat{\mathbf{x}}).
\end{align*}

\section{Details of Our Proposed QR Code Generation Pipelines}

\subsection{Adaptive SRG Detachment via QR Code Error Evaluation}
Considering the inherent error tolerance mechanism of QR codes, we can detach the QR code guidance term when the decoded QR code error is lower than a specific rate during iterative refinement. We define the QR code error evaluation function as:
\begin{align}
    \mathcal{E}(\mathbf{x}, \mathbf{y}) = 
    \frac{1}{N}\sum_{k=1}^{N} \phi(\mathbf{x}_{M_k}, \mathbf{y}_{M_k}),
\end{align}
where $\mathbf{x}$ denotes the decoded image and $\mathbf{y}$ denotes the target QR code.

During each iterative refinement step, we calculate $\mathcal{E}(\mathbf{x}, \mathbf{y})$, if the error is lower than a specific value, we detach the SRG term, reverting to the original score estimation of ControlNet. Please refer from Line 6 to Line 10 in Algo. \ref{algo:qr_code_guidance_1}.

\subsection{One-stage QR Code Generation}
Our end-to-end one-stage generation pipeline is summarized in Algo. \ref{algo:qr_code_guidance_1}.

\begin{algorithm}[H]
    \caption{One-stage QR Code Generation with Iterative Refinement} \label{algo:qr_code_guidance_1}
    \begin{algorithmic}[1] 
        \STATE{\textbf{Input:}
        QR code image $\mathbf{y}$,
        prompt embedding $\mathbf{e}_p$,
        QR code image embedding $\mathbf{e}_\text{code}$,
        UNet $\epsilon_\theta(\cdot, \cdot, \cdot, \cdot)$,
        VAE decoder $\mathcal{D}_{\theta}(\cdot)$,
        sequence $\{\bar{\alpha}_t\}_{t=1}^T$,
        guided weight $\lambda > 0$,
        error rate $\mathcal{E}(\cdot, \cdot)$,
        and QR code error correction capacity $\tau$.
        }
        \STATE{$\mathbf{z}_T \sim \mathcal{N}(\mathbf{0}, \boldsymbol{I})$.}
        \FOR{$t=T$ to $1$}
            \STATE{$\mathbf{z}_{0 \mid t} \leftarrow \frac{1}{\sqrt{\bar{\alpha}_t}}\left(\mathbf{z}_t - \sqrt{1-\bar{\alpha}_t} \epsilon_\theta(\mathbf{z}_t, t, \mathbf{e}_p, \mathbf{e}_\text{code})\right)$.}
            \STATE{$\mathbf{x}_{0 \mid t} \leftarrow \mathcal{D}_{\theta}(\mathbf{z}_{0 \mid t})$.}
            \IF{$\mathcal{E}(\mathbf{x}_{0 \mid t}, \mathbf{y}) \geq \tau$}
                \STATE{$\mathbf{s} \leftarrow \lambda \nabla_{\mathbf{z}_t}\mathcal{L}_\text{SR}(\mathbf{x}_{0 \mid t}, \mathbf{y})$.}
                \STATE{$\hat{\epsilon}_t \leftarrow \epsilon_\theta(\mathbf{z}_t, t, \mathbf{e}_p, \mathbf{e}_\text{code})+\sqrt{1-\bar{\alpha}_t} \mathbf{s}$.}
            \ELSE
                \STATE{$\hat{\epsilon}_t \leftarrow \epsilon_\theta(\mathbf{z}_t, t, \mathbf{e}_p, \mathbf{e}_\text{code})$.}
            \ENDIF
            \STATE{$\mathbf{z}_{t-1} \leftarrow \sqrt{\frac{\bar{\alpha}_{t-1}}{\bar{\alpha}_t}}\left(\mathbf{z}_t - \sqrt{1-\bar{\alpha}_t} \hat{\epsilon} \right) + \sqrt{1-\bar{\alpha}_{t-1}} \hat{\epsilon}$.}
        \ENDFOR
        \STATE{$\mathbf{x}_0 \leftarrow \mathcal{D}_{\theta}(\mathbf{z}_0)$.}
        \RETURN{$\mathbf{x}_0$.}
    \end{algorithmic}
\end{algorithm}

\subsection{Two-stage QR Code Generation}
\subsubsection{SDEdit}
Meng et al. \cite{meng2021sdedit} proposed a training-free, task-agnostic image editing paradigm via Stochastic Differential Equation (SDE). Here we leverage SDEdit to convert the resulting image latent of Stage 1 $\mathbf{z}_0$ to noisy latent $\widetilde{\mathbf{z}}_T$ by adding Gaussian noise according to user-specified $t_0$ for better edit-friendly while ensuring the faithfulness conform to the original latent $\mathbf{z}_0$.
\begin{align}
    \widetilde{\mathbf{z}}_T \sim \mathcal{N}(\mathbf{z}_0, \sigma^{2}(t_0)\mathbf{I}).
\end{align}

In our case, $t_0$ determines the extent of freedom for SRPG, i.e., the lower $t_0$ indicates the less freedom for SRPG to modify the image; the higher $t_0$ indicates the more freedom for SRPG to take effect. In our experiments, we set $t_0 = 1000$.

\subsubsection{Qart}
Qart \cite{qartcodes} is dedicated to blending conventional QR codes with user-specified target patterns via exploiting the padding modules. Here we leverage its capability to blend the reference image from Stage 1 output $\hat{\mathbf{x}}$ and the target QR code $\mathbf{y}$, forming a better baseline QR code $\widetilde{\mathbf{y}}$ for the Stage 2 ControlNet conditioning.

Our end-to-end Two-stage generation pipeline is provided in Algo. \ref{algo:qr_code_guidance_2}.

\begin{algorithm}[H]
    \caption{Two-stage QR Code Generation} \label{algo:qr_code_guidance_2}
    \begin{algorithmic}[1] 
        \STATE{\textbf{Input:}
        QR code image $\mathbf{y}$,
        prompt embedding $\mathbf{e}_p$,
        QR code image embedding $\mathbf{e}_\text{code}$,
        UNet $\epsilon_\theta(\cdot, \cdot, \cdot, \cdot)$,
        VAE encoder $\mathcal{E}_{\theta}(\cdot)$
        VAE decoder $\mathcal{D}_{\theta}(\cdot)$,
        sequence $\{\bar{\alpha}_t\}_{t=1}^T$,
        guided weights $\lambda_1, \lambda_2 > 0$,
        error rate $\mathcal{E}(\cdot, \cdot)$,
        and QR code error correction capacity $\tau$.
        }
        \STATE{
        \tikzmk{begin}
        $\mathbf{z}_T \sim \mathcal{N}(\mathbf{0}, \boldsymbol{I})$.
        \hfill $\triangleright$ Stage 1
        }
        \FOR{$t=T$ to $1$}
        \STATE{$\hat{\epsilon} \leftarrow \epsilon_\theta(\mathbf{z}_t, t, \mathbf{e}_p, \mathbf{e}_\text{code})$.}
            \STATE{$\mathbf{z}_{t-1} \leftarrow \sqrt{\frac{\bar{\alpha}_{t-1}}{\bar{\alpha}_t}}\left(\mathbf{z}_t - \sqrt{1-\bar{\alpha}_t} \hat{\epsilon} \right) + \sqrt{1-\bar{\alpha}_{t-1}} \hat{\epsilon}$.}
        \ENDFOR
        \STATE{$\hat{\mathbf{x}} \leftarrow \mathcal{D}_{\theta}(\mathbf{z}_0)$.
        \hfill 
        \tikzmk{end}
        \boxit{algoblue}
        }
        \STATE{$\widetilde{\mathbf{y}} \leftarrow \operatorname{Qart}(\hat{\mathbf{x}}, \mathbf{y})$.
        }
        \STATE{
        \tikzmk{begin}
        $\widetilde{\mathbf{z}}_T \leftarrow \operatorname{SDEdit}(\mathcal{E}(\hat{\mathbf{x}}))$.
        \hfill $\triangleright$ Stage 2
        }
        \FOR{ $t=T$ to $1$}     
            \STATE{$\widetilde{\mathbf{z}}_{0 \mid t} \leftarrow \frac{1}{\sqrt{\bar{\alpha}_t}}\left(\widetilde{\mathbf{z}}_t - \sqrt{1-\bar{\alpha}_t} \epsilon_\theta(\widetilde{\mathbf{z}}_t, t, \mathbf{e}_p, \mathbf{e}_\text{code})\right)$.}
            \STATE{$\widetilde{\mathbf{x}}_{0 \mid t} \leftarrow \mathcal{D}_{\theta}(\widetilde{\mathbf{z}}_{0 \mid t})$.}
            \IF{$\mathcal{E}(\widetilde{\mathbf{x}}_{0 \mid t}, \widetilde{\mathbf{y}}) \geq \tau$}
                \STATE{$\mathbf{s} \leftarrow \lambda_1 \nabla_{\widetilde{\mathbf{z}}_t}\mathcal{L}_\text{SR}(\widetilde{\mathbf{x}}_{0 \mid t}, \widetilde{\mathbf{y}}) + \lambda_2 \nabla_{\widetilde{\mathbf{z}}_t}\mathcal{L}_\text{LPIPS}(\widetilde{\mathbf{x}}_{0 \mid t}, \hat{\mathbf{x}} )$.}
                \STATE{$\hat{\epsilon}_t \leftarrow \epsilon_\theta(\widetilde{\mathbf{z}}_t, t, \mathbf{e}_p, \mathbf{e}_\text{code})+\sqrt{1-\bar{\alpha}_t} \mathbf{s}$.}
            \ELSE
                \STATE{$\hat{\epsilon}_t \leftarrow \epsilon_\theta(\widetilde{\mathbf{z}}_t, t, \mathbf{e}_p, \mathbf{e}_\text{code})$.}
            \ENDIF            \STATE{$\widetilde{\mathbf{z}}_{t-1} \leftarrow \sqrt{\frac{\bar{\alpha}_{t-1}}{\bar{\alpha}_t}}\left(\widetilde{\mathbf{z}}_t - \sqrt{1-\bar{\alpha}_t} \hat{\epsilon} \right) + \sqrt{1-\bar{\alpha}_{t-1}} \hat{\epsilon}$.}
        \ENDFOR
        \STATE{$\mathbf{x}_0 \leftarrow \mathcal{D}_{\theta}(\widetilde{\mathbf{z}}_0)$.
        \hfill
        }
        \tikzmk{end} \boxit{algogreen}
        \RETURN{$\mathbf{x}_0$.}
    \end{algorithmic}
\end{algorithm}

\section{Post-Processing}
\subsection{Scanning-Robust Projected Gradient Descent (SRPGD)}
In this section, we present a theoretical proof of the convex property of the proposed SRL for post-processing.
This property guarantees the existence of a globally optimal solution and the convergence for SRL. In practice, to leverage the convex property of our SRL for optimization, we remove the early-stopping mechanism of the original $\mathcal{L}_\text{SR}$ as follows:
\begin{align}
\widetilde{\mathcal{L}}_\text{SR}(\mathbf{x}, \mathbf{y}) = \frac{1}{N}\sum_{k=1}^{N} \sum_{(i, j) \in M_k} \mathbf{G}_\sigma(i, j) \cdot \mathbf{E}(i, j).
\end{align}
Then we utilize Projected Gradient Descend (PGD) to update $\mathbf{x}^{t}$ as follows:
\begin{align}
    \mathbf{x}^{t+1} = \operatorname{Proj}_{\mathcal{P}}
    \left( \mathbf{x}^{t} - \eta_t \nabla_{\mathbf{x}^t} \widetilde{\mathcal{L}}_\text{SR}(\mathbf{x}^{t}, \mathbf{y}) \right),
\end{align}
where $\mathcal{P}$ represents the normalized pixel space $[0, 1]^{h \times w \times c}$ and $\eta_t$ be the step size.

\begin{prop}
$\widetilde{\mathcal{L}}_\text{SR}(\mathbf{x}, \mathbf{y})$ is convex function with respect to $\mathbf{x}$.
\end{prop}

\begin{proof}
We first discuss the error of a single RGB pixel $x$ concerning the corresponding target QR code $y$. Then, we extend it pixel-wise throughout the entire image. Let
\begin{align*}
    f(x, y) = \max(1-2\mathcal{G}(x), 0) \cdot y + \max(2\mathcal{G}(x)-1, 0) \cdot (1-y).
\end{align*}
Given $x_1, x_2 \in [0, 1]^{1 \times 1 \times c}$. For all $\alpha \in [0, 1]$, since $\mathcal{G}$ is linear operator, we have
\begin{align*}
\mathcal{G}(\alpha x_1 + (1-\alpha) x_2) = \alpha \mathcal{G}(x_1) + (1-\alpha) \mathcal{G}(x_2).
\end{align*}
The first term can be simplified to
\begin{align*}
    &\max(1-2\mathcal{G}(\alpha x_1 + (1-\alpha) x_2), 0) \\
    &=\frac{1}{2} \left[1-2\mathcal{G}(\alpha x_1 + (1-\alpha) x_2) + |1-2\mathcal{G}(\alpha x_1 + (1-\alpha) x_2)| \right] \\
    &\leq \frac{\alpha}{2}
    (1-2\mathcal{G}(x_1) +
    |1-2\mathcal{G}(x_1)|) +
    \frac{1-\alpha}{2}
    (1-2\mathcal{G}(x_2) +
    |1-2\mathcal{G}(x_2)|) \\
    &=\alpha \max(1-2\mathcal{G}(x_1), 0) +
    (1-\alpha) \max(1-2\mathcal{G}(x_2), 0).
\end{align*}
Similarly, we can simplify the second term. Hence
\begin{align*}
f(\alpha x_1 + (1-\alpha) x_2, y)
\leq \alpha f(x_1, y) + (1-\alpha)f(x_2, y).
\end{align*}
Here, $\mathbf{x}_1, \mathbf{x}_2 \in [0, 1]^{h \times w \times c}$. For all $\alpha \in [0, 1]$, we have
\begin{align*}
&\widetilde{\mathcal{L}}_\text{SR}(\alpha \mathbf{x}_1 + (1-\alpha) \mathbf{x}_2, \mathbf{y}) \\
&= \frac{1}{N} \sum_{k=1}^N \sum_{(i, j) \in M_k} \mathbf{G}_\sigma(i, j) \cdot f(\alpha \mathbf{x}_1(i, j) + (1-\alpha) \mathbf{x}_2(i, j), \mathbf{y}(i, j)) \\
&\leq \frac{\alpha}{N} \sum_{i, j, k} \mathbf{G}_\sigma(i, j) \cdot f(\mathbf{x}_1(i, j), \mathbf{y}(i, j)) + \frac{(1-\alpha)}{N} \sum_{i, j, k} \mathbf{G}_\sigma(i, j) \cdot f(\mathbf{x}_2(i, j), \mathbf{y}(i, j)) \\
&=\alpha \widetilde{\mathcal{L}}_\text{SR}(\mathbf{x}_1, \mathbf{y})
+ (1-\alpha) \widetilde{\mathcal{L}}_\text{SR}(\mathbf{x}_2, \mathbf{y}).
\end{align*}
Therefore, $\widetilde{\mathcal{L}}_\text{SR}(\mathbf{x}, \mathbf{y})$ is convex function with respect to $\mathbf{x}$.
\end{proof}

Since $\mathcal{P}=[0, 1]^{h \times w \times c}$ is a convex set and $\widetilde{\mathcal{L}}_\text{SR}$ is a convex function, $\widetilde{\mathcal{L}}_\text{SR}$ has the global minimum and convergence is guaranteed when performing PGD.

\section{More Experiments}
\subsection{System}
Our code is mainly built based on the Diffusers library \footnote{\url{https://github.com/huggingface/diffusers}} provided by Hugging Face. Tab. \ref{tab:different_parameters} lists the parameters of all other methods used in our experiments; parameters not mentioned are set to their default values.

\begin{table}[]
    \centering
    \caption{Parameters of different methods used in our experiments.}
    \label{tab:different_parameters}
    \begin{tabular}{ll}
        \toprule
        \textbf{Method} & \textbf{Parameters} \\
        \midrule
        QRBTF & Size: 1152px \\
        & Padding ratio: 0.2 \\
        & Anchor style: square \\
        & Correct level: 15\% \\
        \midrule
        QR Code AI Art & ControlNet conditioning scale: 1.1 \\
        & Strength: 0.9 \\
        & Guidance scale: 7.5 \\
        & Sampler: DPM++ Karras SDE \\
        & Seed: 6745177115 \\
        \midrule
        QR Diffusion & QR code weight: 1.65\\
        \midrule
        QR Code Monster & ControlNet conditioning scale: 1.35\\
        \bottomrule
    \end{tabular}
\end{table}

In our experiment, the one-stage required an execution time of 15 seconds, whereas the two-stage took 18 seconds.

\subsection{Prompt Generation}
The 30 prompts we use in our experiment are generated by GPT-4 given the following command: ``Give me 30 prompts for Diffusion Model describing a detailed scene, for example: \texttt{Autumn park, falling leaves, red maple trees, wooden bench, cobblestone path, clear blue sky, squirrel, tranquil, daytime.}''

\begin{lstlisting}
Winter wonderland, fresh snowfall, evergreen trees, cozy log cabin, smoke rising from chimney, aurora borealis in night sky.
Tropical beach at sunset, palm trees, golden sand, calm turquoise sea, hammock, colorful sky, distant sailboat.
Majestic waterfall, lush rainforest, rainbow in the mist, exotic birds, vibrant flowers, serene pool below.
Cherry blossom festival, pink petals floating in the air, traditional lanterns, peaceful river, people in kimonos, sunny day.
Ancient city ruins at dawn, misty mountains in the background, wildflowers, crumbling stone structures, first light of day.
Lavender fields at sunset, rows of purple, golden hour light, old farmhouse, bees buzzing, tranquil countryside.
Moonlit garden, reflecting pond, white marble statues, night-blooming flowers, wrought iron bench, starry sky.
Snow-covered village, holiday lights, decorated pine trees, ice skating pond, families enjoying, twilight.
Desert oasis at midday, palm trees, clear blue water, sand dunes, camels resting, vibrant sky.
Mountain peak at sunrise, sea of clouds below, rugged terrain, first light hitting the summit, sense of achievement.
Old European town square, cobblestone streets, cafe terraces, flowering balconies, gothic cathedral, bustling morning.
Underwater coral reef, colorful fish, sunbeams through water, sea turtles, diverse marine life, peaceful exploration.
Forest clearing at night, fireflies, full moon, ancient oak tree, soft grass, mystical ambiance.
Zen garden at dawn, raked sand patterns, stone path, bamboo fence, calm pond, serene meditation spot.
Vineyard hills at harvest time, rows of grapevines, rustic winery, mountains in the distance, sunny afternoon.
Northern lights over a frozen lake, snow-covered pines, clear night sky, reflection on ice, isolated cabin.
Sunflower field at midday, blue sky with fluffy clouds, endless rows of yellow, picturesque farmhouse.
Grand library, towering bookshelves, spiral staircase, soft sunlight through stained glass, quiet study corners.
Mediterranean seaside town, white-washed buildings, blue-domed churches, fishing boats, vibrant market, sunny day.
Foggy London street, vintage lampposts, double-decker bus, historic buildings, cobblestone pavement, early morning.
Serene monastery in the mountains, monks in meditation, tranquil gardens, mist rolling over peaks, sense of peace.
Blooming orchard in spring, rows of fruit trees, petals in the air, picnic under blossoms, clear day.
Rainforest canopy walkway, lush greenery, bird's eye view, exotic wildlife, adventure in nature.
Rooftop garden in the city, skyline view, flowering plants, comfortable seating, sunset ambiance.
Arctic expedition, icebergs, polar bears, aurora in the sky, rugged icebreaker ship, adventure in the cold.
Traditional Japanese tea garden, koi pond, red bridge, cherry blossoms, tea ceremony, peaceful afternoon.
Old Western ghost town at dusk, abandoned buildings, dusty streets, setting sun, sense of history.
Cliffside lighthouse at stormy sea, waves crashing, beacon of light, rocky shore, dramatic weather.
Futuristic city at night, neon lights, flying cars, towering skyscrapers, advanced technology, vibrant life.
African savannah at golden hour, acacia trees, grazing elephants, distant mountains, wild beauty.
\end{lstlisting}

\subsection{Influences On Devices}
\begin{table}[]
    \caption{Scanning success rate.}
    \label{tab:different_device}
    \centering
    \begin{tabular}{cccc}
        \toprule
         & iPhone 13 & Pixel 7 & QR Verify \\
         \midrule
        One-stage & 100.00\% & 91.67\% & 96.67\% \\
        Two-stage & 96.67\% & 88.00\% & 100.00\% \\
        \bottomrule
    \end{tabular}
\end{table}

We further analyze the scannability of our methods using three different QR code scanners: the built-in scanner on the iPhone 13, the built-in scanner on Pixel 7, and the software scanner `QR Verify'\footnote{\url{https://github.com/antfu/qr-verify}}, which is powered by the WeChat decoding algorithm. 30 aesthetic QR codes used in our experiment are scanned 10 times, and we calculate the percentage of successful scans (Tab. \ref{tab:different_device}).

\subsection{Influences of Scanning Angles}
\begin{figure}
    \centering
    \includegraphics[width=.9\linewidth]{figures/Supplementary/flip.png}
    \caption{Visualization in different scanning angles of QR code using CSS. Zoom in for better scannability.}
    \label{fig:different_angle}
\end{figure}

We also analyze the scannability under different scanning angles. Two QR codes, randomly chosen from our one-stage and two-stage results, are tested. We use CSS to rotate the QR code by 30, 45, 60, 75, and 90 degrees (Fig. \ref{fig:different_angle}). A QR code is considered scannable if it can be scanned within 3 seconds. As shown in Tab. \ref{tab:different_angles}, our QR codes can be scanned even at a 60-degree angle.

\begin{table}[]
    \centering
    \caption{Scannability of different angles.}
    \begin{tabular}{cccccc}
        \toprule
         & $30^\circ$ & $45^\circ$ & $60^\circ$ & $75^\circ$ & $90^\circ$ \\
         \midrule
         One-stage & \CheckmarkBold & \CheckmarkBold & \CheckmarkBold & \XSolidBrush & \XSolidBrush \\
         Two-stage & \CheckmarkBold & \CheckmarkBold & \CheckmarkBold & \XSolidBrush & \XSolidBrush \\
         \bottomrule
    \end{tabular}
    \label{tab:different_angles}
\end{table}

\section{User Study}
\subsection{Privacy Issues}
We obtain all the users' consent before participating in the survey, disclose the data processing policy including immediate destruction after the statistic report, and avoid collecting personal sensitive data. In addition, users are informed they can quit the survey anytime.

\subsection{Details}

\begin{figure}
\centering
\begin{subfigure}{.5\textwidth}
  \centering
  \includegraphics[width=.9\linewidth]{figures/Supplementary/city.png}
  \caption{}
  \label{fig:user_study_aesthetic_1}
\end{subfigure}%
\begin{subfigure}{.5\textwidth}
  \centering
  \includegraphics[width=.5\linewidth]{figures/Supplementary/forest.png}
  \caption{}
  \label{fig:user_study_aesthetic_2}
\end{subfigure}
\caption{(a) A sample question on aesthetics with and without Scanning-Robust Loss. (b) A sample question on aesthetics with different methods.}
\label{fig:user_study_details}
\end{figure}

Fig. \ref{fig:user_study_details} is an example of the first and second questions in our questionnaire. Participants will see three or four enhanced QR codes (one of them is generated using our method) and be asked to rank A, B, C, and D according to the order of their perceived aesthetic appeal.

\begin{figure}
    \centering
    \includegraphics[width=.6\linewidth]{figures/Supplementary/snow.png}
    \caption{A sample question on aesthetic QR code before (left) and after (right) post-processing.}
    \label{fig:user_study_post-processing}
\end{figure}

Fig. \ref{fig:user_study_post-processing} is an example of the third question in our questionnaire. Participants will see two QR codes: one that is unscannable due to a high error rate and another post-processed to be scannable. They are asked whether they can accept the loss of aesthetic appeal caused by the post-processing correction.

\subsection{Rank Calculation}
To evaluate the user study's results, we calculate each weighted average rank by summing up all ranks given and dividing by the number of participants. Suppose 20 participants rank a QR code as 1, 10 participants rank it as 2, and 100 participants rank it as 3, the average rank of that QR code can be calculated as:

\begin{align}
\frac{1 \times 20 + 2 \times 10 + 3 \times 100}{130} = 2.615 .
\end{align}

\subsection{Responses}
\begin{figure}
\centering
\begin{subfigure}{.5\textwidth}
  \centering
  \includegraphics[width=.7\linewidth]{figures/Supplementary/compare_1.png}
  \caption{Weighted Rank.}
  \label{fig:user_study_aesthetic_3}
\end{subfigure}%
\begin{subfigure}{.5\textwidth}
  \centering
  \includegraphics[width=.8\linewidth]{figures/Supplementary/compare_2.png}
  \caption{Weighted Rank.}
  \label{fig:user_study_aesthetic_4}
\end{subfigure}
\caption{(a) The weighted ranks in questions about aesthetics with and without Scanning-Robust Loss. (b) The weighted ranks in questions about aesthetics with different methods.}
\label{fig:test}
\end{figure}

Fig.~\ref{fig:test} (a) shows the result of participants' preference for aesthetics with and without Scanning-Robust Loss (SRL). Participants are asked to rate two sets of three aesthetic QR codes, a QR Code Monster (without SRL), a QR code generated by our one-stage pipeline, and a QR code generated by our two-stage pipeline, from 1 (the highest) to 3 (the lowest). Regarding these QR codes, the result shows that our pipelines have a minimal gap compared to QR Code Monster, with negligible impact on aesthetics. 
Fig.~\ref{fig:test} (b) shows the participants' preference for aesthetics on four methods: QR Diffusion, QR Code AI Art, QRBTF, and two-stage. They are asked to rate two sets of four aesthetic QR from 1 (the highest) to 4 (the lowest). In addition to defeating QR Diffusion and QR Code AI Art, our method also shows strong competitiveness against QRBTF by demonstrating a close average rank.

\section{More Qualitative Results}
We use GPT-4 to generate 10 prompts for more qualitative results (Fig. \ref{fig:more}).
\begin{figure}
    \centering
    \includegraphics[width=\linewidth]{figures/Supplementary/more_graph.png}
    \caption{More qualitative results and corresponding prompts.}
    \label{fig:more}
\end{figure}

\section{Limitation and Future Work}
Though our approach showcases impressive aesthetic QR code generation capability compared to pre-dominant methods, it sometimes falls short of ensuring 100\% scannability and requires some extent of hyperparameter tuning for better results, therefore, we introduce post-processing to polish the results. Future work will focus on improving our approach to be a hyperparameter-insensitive end-to-end pipeline that does not rely on post-processing. In addition, we can further enhance the controllability via image-to-image methodologies for more personalized aesthetic QR code generation.

\section{Societal Impacts}
Our proposed approach might be maliciously exploited for phishing, spam, and false or inappropriate content propaganda, this issue can be addressed by user-input pre-checking such as URL filtering, prompt blacklist, etc.
